# Supplementary material for: Spinner: Automated Dynamic Command Subsystem Perturbation
Source: arXiv:2105.00391 source file (2021-09-16)
Supplement: Supplementary file 2 [file table_appendix_sinks.tex]

\begin{table}[h]
	\centering
	\caption{Sink Functions}
	\vspace{-1em}
	\label{table:additional_sink_functions}
	
\resizebox{1.0\columnwidth}{!}{%	

\begin{tabular}{l c c} % 4 columns
	\toprule
	{\bf Sink Functions} & 
	{\bf Subsystem} &
	{\bf Language}
	\\ 
	\midrule
	
	{\tt mysqli::multi\_query()}, {\tt mysqli::prepare()},  &
	\multirow{3}{*}{MySQL} &
	\multirow{3}{*}{PHP} \\ 
	
	{\tt mysqli::real\_query()}, {\tt mysqli::select\_db()}, &
	&
	 \\ 
	
	{\tt mysqli::send\_query()} &
	&
	\\ \midrule

	{\tt mysql\_create\_db()}, {\tt mysql\_drop\_db()}, &
	\multirow{3}{*}{MySQL} &
	\multirow{3}{*}{C/C++} \\
	{\tt mysql\_query()}, {\tt mysql\_real\_query()}, &
	 &
	 \\
	{\tt mysql\_select\_db()}  &
	 &
	 \\ \midrule

	{\tt sqlite\_array\_query()}, {\tt sqlite\_exec()}, &
	\multirow{4}{*}{SQLite} &
	\multirow{4}{*}{PHP} \\ 
	{\tt sqlite\_open()}, {\tt sqlite\_query()}, & & \\ 
	{\tt sqlite\_popen()}, {\tt sqlite\_single\_query()}, & & \\ 
	{\tt sqlite\_unbuffered\_query()} & & \\ \midrule
	
	{\tt sqlite3\_get\_table()}, {\tt sqlite3\_exec()}, &
	\multirow{3}{*}{SQLite} &
	\multirow{3}{*}{C/C++} \\ 
	{\tt sqlite3\_prepare()$^1$}, {\tt sqlite3\_prepare16()$^2$},  & & \\ 
	{\tt sqlite3\_open()$^3$} & & \\ \midrule

	{\tt libxml.parseXmlString()}, {\tt parser.parseString()}, & \multirow{2}{*}{XML} & \multirow{2}{*}{JavaScript} \\ 
	{\tt parser.push()}, {\tt element.find()}, {\tt element.get()} & & \\ \midrule

	{\tt callbacks.StartDoctypeDecl()}, {\tt parser:parse()} & XML & Lua \\

	\bottomrule

	\multicolumn{3}{l}{$1$: inlcuding \code{sqlite3\_prepare\_v2()},  \code{sqlite3\_prepare\_v3()}.} \\
	
	\multicolumn{3}{l}{$2$: inlcuding \code{sqlite3\_prepare16\_v2()},  \code{sqlite3\_prepare16\_v3()}.} \\
	
	\multicolumn{3}{l}{$3$: inlcuding \code{sqlite3\_open16()}, \code{sqlite3\_open\_v2()}.}

\end{tabular}

}
%\caption{Database Sink Functions}
\vspace{-1em}
\end{table}
